# Supplementary material for: On the Complexity of Simple and Optimal Deterministic Mechanisms for an Additive Buyer
Source: arXiv:1702.07032 source file (2017-07-14)
Supplement: Supplementary file 1 [file appendix.tex]

% !TEX root = main.tex
\newpage  

\section{\#P-hardness of \texorpdfstring{COMP$^*$}{COMP*}}\label{appendix1}

We give a polynomial-time reduction from COMP to COMP$^*$ (i.e., COMP with two extra conditions on $B$ and $W$).
Let $(B,W,t)$ be an input to the original COMP problem, where $B=\{b_1,\ldots,b_n\}$
  with $b_1,\ldots,b_n\in [0:2^n]$, $W\subset [n]$ with $|W|=n/2$, and $w=\sum_{i\in W} b_i$.
We first construct from $B$ a new set $B'$ of $4n$ integers between $0$ and $2^{4n}$:
\begin{enumerate}
\item $B'$ contains $n$ integers $2^{2n}+b_i$, $i\in [n]$;
\item $B'$ contains $2^{4n}$ (as the largest integer in $B'$) and $3n/2$ copies of $2^{3n}$;
\item The rest of $3n/2-1$ integers of $B'$ are all $0$ (so the smallest two integers in $B'$ are $0$).
\end{enumerate}
The new set $W'$ contains $2n$ integers from $B'$: the $3n/2$ copies of $2^{3n}$
  and each of $2^{2n}+b_i$, $i\in W$. Let 
$$
w'=\sum_{b\in W'} b=(3n/2)\cdot 2^{3n}+ (n/2)\cdot 2^{2n}+w\quad\text{and}\quad
t'=\binom{4n-1}{2n-1} +t.
$$

We show that $B'$ and $W'$ satisfy the two extra conditions.
For the first part note that $\sum_{b\in S} b>w'$ for any subset $S$ that contains the
  largest integer $2^{4n}$.
On the other hand, if $S$ is a $2n$-subset of $W'$ that does not contain $2^{4n}$ but contains 
  at least one $0$, then we have (using $b_i\le 2^n$ for all $i\in [n]$)
$$
\sum_{b\in S} b\le (3n/2)\cdot 2^{3n}+(n/2-1)\cdot (2^{2n}+2^n)<w'.
$$ 

Let $S$ be a $2n$-subset that satisfies $\sum_{b\in S} b\ge w'$.
Then either i) $S$ contains $2^{4n}$, or ii) $S$ contains all the $3n/2$ copies of $2^{3n}$
  and a subset of $n/2$ integers $2^{2n}+b_i$, with the sum of the latter 
  being at least $(n/2)\cdot 2^{2n}+w$.
This then implies that $(B,W,t)$ is a yes-instance if and only if $(B',W',t')$ is a yes-instance.
It follows that COMP$^*$ is also \#P-hard.
